# Supplementary material for: Understanding Physical Dynamics with Counterfactual World Modeling
Source: arXiv:2312.06721 source file (2024-07-22)
Supplement: Supplementary file 1 [file mathematical_derivations.tex]

\section{Mathematical formulation of vision structure extraction}
In this section we formally define the operations used to extract keypoints, optical flow, and Spelke object segments. For clarity, this section is largely a recapitulation of the contents in the paper \cite{bear2023unifying}, but it is presented here for readers' convenience. We refer the readers to Section 2 and 3 of the paper \cite{bear2023unifying} for further details.

\subsection{Keypoints}
In Section 3.3 of the main text we define a query for extracting keypoints from a given input frame pair, as originally described in \cite{bear2023unifying}. Here we formally define that procedure. Let $\Psi$ be the CWM predictor. Suppose we are given an input frame pair $x_1, x_2$, an initial patch index set $p_0$, and an integer $k$.  The \emph{$k$-subsequent keypoint set} for $x_2$ from $p_0$ is
$$K(x_1, x_2, p_0, k) = \argmin_{\{p \,\subset\,\mathcal{I} - p_0 \,|\, |p| = k\}} \mathcal{L}(\Psi(x_1, {x_2}_{p_0 \cup p}), x_2)$$ 
where ${x_2}_{p_0 \cup p}$ denotes the patches of $x_2$ at the patch index set $\,p_0 \cup p$ \cite{bear2023unifying}. Ideally it would be possible to efficiently compute $K(x_1, x_2, p_0, k)$ directly for large $k$.  However, this is in general an intractable optimization problem.  Instead, it is substantially more efficient (though still rather inefficient in absolute terms) to take a greedy approach by finding one keypoint at a time and iterating, e.g. defining 
$$k_i = k_{i-1} \cup K(x_1, x_2, k_{i-1}, 1),\quad \text{where } k_0 = \varnothing.$$

\subsection{Flow as derivatives }
Section 3.3 also describes the counterfactual query for extracting optical flow at a pixel location $i$, as originally described in \cite{bear2023unifying}. The querying procedure starts by injecting a perturbation $\delta$ at location $i$ of the first frame $x_1$, and then inspects how the perturbation is propagated onto the next frame $x_2$ using the predictor $\Psi$. This procedure has one potential failure mode: the perturbed frame $x_1^{i}$ could be out of distribution for $\Psi$. This could happen when the perturbation is either too large so that it looks ``fake'' rather than like a piece of the surface it is placed on, or too small so that it cannot be detected and moved accurately.
This is naturally addressed by considering $\Psi$'s \textit{infinitesimal responses to infinitesimal perturbations} -- which are exactly the \textit{derivative} of the prediction model \cite{bear2023unifying}:
% 1) If we unmask a patch in the next frame  $x_2$ which is the destination location of the perturbation $\delta \i $ from the current frame $x_1$ then the algorithm fails. This can easily be addressed by running the query several times, unmasking a different set of patches in $x_2$ each time and taking their average result, removing samples where $|\hat{\delta}_p| / | \delta_{\i}| \ll 1$. 2) 
\vspace{-0.5cm}

\begin{align}
&\textbf{Normalized Perturbation Response at i} \nonumber \\
%\lim_{\delta \i \rightarrow 0} \frac{|\hat{\delta}_{\i}|}{|\delta \i|}  & \nonumber \\
& = \lim_{\delta \rightarrow 0} \frac{|\tilde{x}^{i}_{2} - x_{2}|}{|x^{i}_1 - x_1|} \nonumber \\
& = \nabla_{x}\Psi \bigg|_{i} 
\end{align}

To simultaneously estimate optical flow at all locations in an $H \times W$ frame pair, we can compute the Jacobian of $\Psi$.
This is a four-tensor $\mathcal{J}\Psi$ of shape $H \times W \times H \times W$, which assigns to element $(i, j, k, l)$ the predictor's change in output at location $(k,l)$ in the second frame due to an infinitessimal change at location $(i, j)$ in the first frame. Applying this derivative implementation to the algorithm above,
\begin{equation}
    \textbf{flow}(k, l) = 
    \begin{cases}
        \text{undefined}, &\text{if } \mathcal{J}\Psi(i',j',k,l)| \ll 1 \\
        (k,l)-(i', j'), &\text{otherwise} \\
    \end{cases}
\end{equation}

where $(i', j') = \argmax_{i,j}\mathcal{J}\Psi(i,j,k,l)$. Note that this method detects disocclusion at the location where flow is undefined. This method does not detect occlusion, since no perturbation at any location in the first frame will cause a response at a point that becomes disoccluded in the second frame.

Because it is a tensorial operation, the derivative formulation of the counterfactual enables a more efficient parallel computation for flow than serial finite perturbations, implemented practically using Jacobian-vector products available in autograd packages such as PyTorch or Jax.

\subsection{Spelke affinities as derivatives}

As described in \cite{bear2023unifying}, while it is impossible to pin down general definitions of “object” or “segmentation”, an early developmental shift in perception suggests the practically useful notion of a Spelke object. Work by cognitive scientist Elizabeth Spelke and her colleagues revealed that babies begin life grouping separated visual elements into objects only when they are moving in concert; it is not until they are almost a year old that babies expect, for example, two stationary toys resting on each other to be independently movable \cite{spelke1990principles}. We therefore define a Spelke object as \textit{a collection of physical stuff that moves together during commonplace physical interactions} \cite{bear2023unifying}. This includes common physical objects like cell phones, wallets, coffee cups, dogs, people, and cars, as well as complex novel objects from semantically unnamed categories that nonetheless can be seen to move coherently.

Inspired by the notion of Spelke object, we relax the definition of “object” or “segmentation” to pairwise affinities between scene elements, which is high for two elements that often move together and low otherwise. It is the set of \textit{possible} affinities -- that is, how often would two elements move together across a wide variety of dynamics -- that supports a good representation of how objects should be grouped and how they can behave.

This relaxation of segments to pairwise affinities allows the above algorithm to be interpreted as another \textit{derivative} of $\Psi$ (combined with the optical flow estimator.)
We define the \textit{Spelke affinity} between two points $i$ and $j$ to be the response in the flow estimate at $j$ given a counterfactual change in the flow estimate at $i$. 
For any input frame pair $(x, y)$ (including frame pairs for which $x = y$, i.e. static images), in the infinitesimal limit of the motion counterfactual size, we can write the Spelke affinity between $i$ and $j$ as $\partial_{y_i}\textbf{Flow}(x, y)[j]$, or in tensorial form:
\begin{equation}
\textbf{SpelkeAffinity}[x] = \nabla_{y} \textbf{Flow}[x, y].
\end{equation}
Even when objects can undergo complex motion, such that pairs of points sometimes move together and sometimes do not, partial or complete Spelke affinities can be converted to (binarized) estimated segments via grouping operation such as Kaleidoscopic Propagation introduced in~\cite{chen2022unsupervised}.
Besides providing an efficient method for segmenting Spelke objects, this derivative construction conceptually unifies segmentation with optical flow estimation -- illustrating that two apparently distinct computer vision tasks emerge, zero-shot, from the same unsupervised model.
