# Supplementary material for: Understanding Physical Dynamics with Counterfactual World Modeling
Source: arXiv:2312.06721 source file (2024-07-22)
Supplement: Supplementary file 2 [file supp_jacobian_cosine_flow_comparison.tex]

\begin{figure*}
  \centering
  \includegraphics[width=0.99\linewidth]{figures/jacobian_cosine_similarity_copy_without_illustrator.pdf}

  \caption{\label{first}\textbf{Comparison between the pertubation method and cosine approximation} We compare the full perturbation-based optical flow extraction algorithm introduced in the main paper against the cosine-similarity approximation given in Algorithm  \ref{algorithm:cosine_flow}. The fidelity of the approximation method is very close to the complete flow estimate, while benefiting from much lower computational complexity.} 
  
  \label{fig:supp_jacobians_cosine_comparison}
\end{figure*}
