# Supplementary material for: Understanding Physical Dynamics with Counterfactual World Modeling
Source: arXiv:2312.06721 source file (2024-07-22)
Supplement: Supplementary file 3 [file flow_supp.tex]

\begin{table}[t]
  \centering
  \footnotesize
  \begin{tabular}{lc}
    \toprule
    Method & epe $\downarrow$ \\
    \midrule
    \multicolumn{2}{l}{\textit{Methods trained on synthetic data}} \\
    \midrule
    PWCNet~\cite{sun2018pwc} & 2.288 \\
    SPyNet~\cite{ranjan2017optical} & 4.162 \\
    SMURF-Sintel~\cite{stone2021smurf} & 1.741 \\
    RAFT-Sintel~\cite{teed2020raft} & \textbf{1.476} \\
    \midrule
    \multicolumn{2}{l}{\textit{Methods trained on real data}} \\
    \midrule
    RAFT-KITTI~\cite{teed2020raft} & 4.356 \\
    SMURF-KITTI~\cite{stone2021smurf} & 3.604 \\
    \midrule
    CWM & 4.981 \\
    \bottomrule
  \end{tabular}
  \caption{Additional results \\ on SPRING benchmark}
  \label{tab:flow_spring_supp} 
\end{table}
